# Supplementary material for: Nontrivial electrophoresis of silica micro and nanorods in a nematic liquid crystal
Source: arXiv:2204.11195 source file (2022-04-24)
Supplement: Supplementary file 1 [file SUPPLEMENTARY.pdf]

Supplementary Information for

# Nontrivial electrophoresis of silica micro and nanorods in a nematic liquid crystal

*Muhammed Rasi M[1], Archana S[1], Ravi Kumar Pujala[2] and Surajit Dhara[1*]*

*[1]School of Physics, University of Hyderabad, Hyderabad-500046, India*

*[2]Department of Physics, Indian Institute of Science Education and Research, Tirupati, Andhra Pradesh 517505, India*

## Frequency dependence of electrophoretic velocities of nano and micro-rods

We have measured the frequency dependent propulsion velocity of the rods. Figure 9 shows the frequency dependence of the velocity of both the nano- and micro-rods in the frequency range of 10-120 Hz. It increases rapidly with frequency to a peak velocity and then de-creases. Overall the frequency response of the silica rods shows a behavior similar to that of the spherical particles. According to the induced charge electrophoresis, the frequency dependence of velocity of a spherical particle is given by

$$V_i(\omega)=V_i^0\frac{\omega^2\tau_e^2}{(1+\omega^2\tau_p^2)(1+\omega^2\tau_e^2)} \quad \text{.........} \quad (1)$$

Where $\omega = 2\pi f$, $\tau_p = \lambda_D L/2D$ is the particle charging time and $\tau_e = \lambda_D d/2D$ is the electrode charging time. The experimental data is fitted with Eq. (1), and the continuous red lines show the best fits to the data. The fit parameters are $\tau_p$ =0.051 s and $\tau_e$ =0.021 s for the nanorods and $\tau_p$ =0.049 s and $\tau_e$ =0.017 s for the micro-rods.

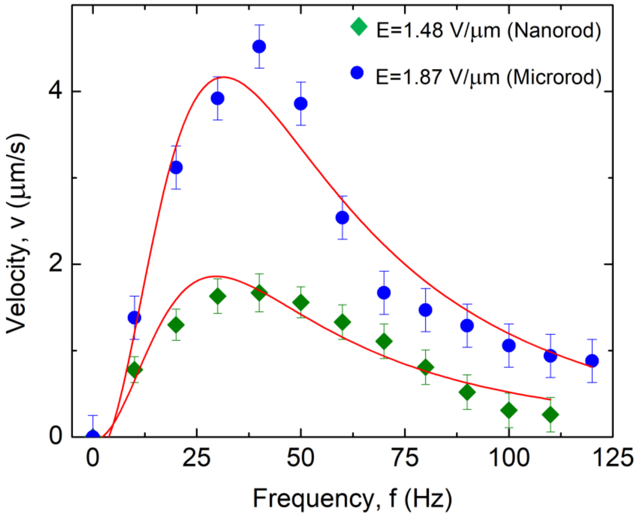


*FIG.1: Frequency dependence of velocity of nanorods (solid circles) and microrods (solid diamonds). Solid curves are best fits to Eq. (1).*

Description of movies

Movie-S1 (Movie S1.avi): A microrod oriented perpendicular to the director (in a cell with in-plane stripe electrodes) moving at angle with the rubbing direction under increasing DC electric field (1-12 V/$\mu m$). The in-plane electric field is applied perpendicular to the rubbing direction.

Movie-S2 (Movie S2.avi): Effect of AC electric field (50Hz, 1.6 V/$\mu m$) on a silica microrod in MLC-6608. Video recorded with additional λ-plate in POM.

Movie-S4 (Movie S3.avi): Effect of AC electric field ((50Hz, 1.8 V/$\mu m$)) on a silica nanorod in MLC-6608. Video recorded with additional λ-plate in POM.
